# Supplementary material for: DINOv2: Learning Robust Visual Features without Supervision
Source: arXiv:2304.07193 source file (2024-02-02)
Supplement: Supplementary file 1 [file supp-results.tex]

\section{Evaluation Implementation Details}

\subsection{Baseline Configurations}

\subsection{ImageNet Classification}

\subsubsection{Linear Classification}
For linear classification, we apply the iBOT protocol. 
We instantiate 52 linear classifiers with the following grid of parameters: use the class token from the [1 or 4] last blocks, [use or don't use] the average of the patch tokens, use a learning rate in [1e-5, 2e-5, 5e-5, 1e-4, 2e-4, 5e-4, 1e-3, 2e-3, 5e-3, 1e-2, 2e-2, 5e-2, 1e-1]. 
We train all of them simultaneously with SGD on the linear probing dataset (usually Imagenet-1k), with learning rate following a cosine schedule, using only random resized crop and horizontal flip as data augmentations, and retrieve the best classifier in the grid. 
We train the linear classifier for 12500 iterations, for the results shown in Table~\ref{tab:lin-inet1k} of the main text.

\subsubsection{Finetuning}
We finetune our models on ImageNet-1k using the recipe presented in DeiT III \cite{touvron2022deit}. 
It uses the Three-augment transform with random resized crop, without erasing, and with mixup alpha set at 0.8, cutmix alpha set at 1.0 and color jitter probabilities at 0.3.
We use the binary cross-entropy loss as suggested by \cite{wightman2021resnet}, with label smoothing at 0.1.
The optimization is carried out with the AdamW~\cite{loshchilov2018fixing} optimizer during 50 epochs, where the learning rate follows a cosine-annealing schedule, with a linear warmup of 5 epochs.
The weight decay is of 0.05, and the layer decay is set at 0.7 for all models (this rather high layer decay - meaning that only shallow transformer blocks are optimized - can be explained by the fact that the SSL pre-training creates a strong backbone). 
The progressive stochastic drop path rate is set at 0.3, 0.4, 0.5 for ViT-L, ViT-H, ViT-G respectively.

\subsubsection{Robustness Analysis}
To verify the robustness of our models to out-of-distribution data,
we evaluated our features on ImageNet-A(dversarial) (\texttt{Im-A})~\cite{hendrycks2021natural}, ImageNet-R(endition) (\texttt{Im-R})~\cite{hendrycks2021many},
ImageNet-C(orruptions) (\texttt{Im-C})~\cite{hendrycks2018benchmarking},
ImageNet-Sketch (\texttt{Sketch})~\cite{wang2019learningrobust},
ImageNet ReaL (\texttt{Real})~\cite{beyer2020imagenetreal} and
ImageNet-V2 (\texttt{V2})~\cite{recht2019imagenetv2}. 
We report the mean corruption error (\texttt{mCE}) on ImageNet-C, ReaL accuracy on ImageNet ReaL and top-1 accuracy on the rest of the datasets.

\subsection{Instance-level Recognition}
On the revisited Oxford and Paris datasets, we directly apply a $k$-NN search on the frozen features and report mean average precision (mAP) for the medium (M) and hard (H) splits. 
On the Met dataset, we use the evaluation protocol and code of the authors. 
This is similar to the nearest neighbor recognition protocol with L2-normalization, cosine-similary-based $k$-NN retrieval followed with a softmax. 
There are however two differences: features are whitened on the train split before retrieval and a grid search is conducted to optimize the parameters of the classifier using the validation split. 
PCA dimensionality reduction is not applied to our embeddings as it degrades performance. 
For completeness, we also include global average precision (GAP) metrics. 
On the AmsterTime dataset, performance is reported on the main task of dataset, bidirectional retrieval of old and new images. 
We again use the procedure and code of the authors, which builds a nearest-neighbor classifier on top of our frozen features. 
The mAP numbers are obtained using cosine similarity and a fixed $k = 128$ to match the parameters applied by the authors.

\subsection{Monocular depth estimation}
We follow the evaluation protocol of BinsFormer~\cite{li2022binsformer} and report the RMSE of our depth prediction.
We use a ViT backbone and plug a linear or a DPT decoder~\cite{ranftl2021vision} on top of the ViT patch tokens. We select the patch tokens from layers $l=\{5, 12, 18, 24\}$ for ViT-L, $l=\{10, 17, 23, 32\}$ for ViT-H and $l=\{10, 20, 30, 40\}$ for ViT-G as an input for our linear and DPT head. We bi-linearly upsample the patch tokens by a factor of 4 to increase the resolution of the linear decoder output then concatenate the 4 layers along with the CLS token of the same layers for our linear decoder giving us an input dimension of $4 \times 2 \times \text{embed dim}$. For the DPT decoder we reassemble those tokens following standard DPT pipeline.
We use a classification task instead of a regression for our linear head by dividing the depth prediction range in 256 uniformly distributed bins and use a linear normalization following AdaBins~\cite{bhat2019adabins}.
We train our models by freezing all parameters from the ViT backbone and use a batch size of 16 and a learning rate of $1e-4$ for 38.4k iterations on a single node of 8 GPUs.

\subsection{Image Segmentation}
\subsubsection{Linear}
For the linear segmentation evaluation, we concatenate the patch tokens of the last 4 blocks of the transformer, before applying a batch normalisation and a linear classification layer. The patch classification probabilities are then upsampled to pixel classifications through a bilinear layer. During training of the linear layer, the images have their smallest side resized to a random size in the range $[256,1024]$, then cropped and padded to 512x512. During testing, the images have their smallest side resized to 512, then we use a sliding window procedure to extract crops of size 512x512 with stride 341. Each of these crops is fed through the model to obtain predictions, then the predictions are averaged on overlap regions. We train the model for 40k iterations with $lr_{base}=1e-3$, $wd=1e-4$ and $momentum=0.9$. The lr follows a polynomial schedule: $lr=lr_{base} \cdot (1-\frac{iter}{max\_iter})^{0.9}$.

\subsubsection{Multiscale}
For the multiscale evaluation, we reuse the same setup as for the linear, with a few modifications. During training, the images are resized to a random size in $[640, 1920]$ before being cropped to 640x640. During testing, the images are resized to each size in ${640, 845, 1107, 1459, 1920}$, converted to crops with a sliding window of size 640x640 and stride 320, and finally the predictions are averaged so that each scale has the same weight in the final predictions.

\subsubsection{Frozen backbone in ViT-adapter + mask2former}
For this evaluation we reuse the configuration of the official ViT-adapter \cite{chen2022vision} in which the weights of the ViT backbone are initialized with our pretrained weights. These backbone weights are frozen, i.e. not trained. We then train the SPM, injectors, extractors and the mask2former with a 40k iteration schedule and default hyperparameters.
